# Supplementary material for: Efficient Binary Embedding of Categorical Data using BinSketch
Source: arXiv:2111.07163 source file (2021-11-13)
Supplement: Supplementary file 1 [file appendix.tex]

%\section{Appendix}
%\subsection{Reproducibility details for baseline algorithms}
We first give implementation details of the baseline algorithms as follows:
\begin{enumerate}
 \item  We used our own implements for \tsketch, ~ {Feature Hashing (FH)}~\cite{WeinbergerDLSA09} and   {SimHash (SH)}\cite{simhash} algorithms. We give its link via an anonymous repository here \footnote{\url{}}. \todo{To update the new code repo},
 \item for  {Kendall rank correlation coefficient}\cite{kendall1938measure} we use \texttt{pandas data frame implementation}\footnote{\url{https://pandas.pydata.org/pandas-docs/stable/reference/api/pandas.DataFrame.corr.html}}, 
 \item for {Latent Semantic Analysis (LSA)}~\cite{LSI}, {Latent Dirichlet Allocation (LDA)}\cite{LDA}, {Non-negative Matrix Factorization (NNMF)}\cite{NNMF}, and  vanilla {Principal component analysis (PCA)}, we use the implementation available \texttt{sklearn.decomposition} library \footnote{\url{https://scikit-learn.org/stable/modules/classes.html\#module-sklearn.decomposition}},
 \item for {Multiple Correspondence Analysis (MCA)}\cite{MCA}, we use the following implementation\footnote{\url{https://pypi.org/project/mca/}},
 \item finally for $\chi^2$-{feature selection} \footnote{\url{https://scikit-learn.org/stable/modules/generated/sklearn.feature_selection.chi2.html\#}}\cite{chi_square} and  {Mutual Information based feature selection}\cite{MI}\footnote{\url{https://scikit-learn.org/stable/modules/generated/sklearn.feature_selection.mutual_info_classif.html}} we use the implementation available at \texttt{sklearn.feature\_selection} library.
 \end{enumerate}
\noindent\textbf{Limitation of baseline algorithms for inclusion in end tasks:} We include $\chi^2$-{feature selection}, and   {Mutual Information based feature selection} algorithm only in the classification tasks for comparison as they require labeled data for feature selection. PCA, MCA and LSA can reduce the data dimension up to the minimum of the number of data points
and the original data dimension. We summarise the characteristic of all the baseline algorithms in Table~\ref{tab:baseline_characteristic}.

% \hspace*{-1cm}
% \setlength{\tabrowsep}{6pt}
\begin{table*}
\centering
\caption{\footnotesize{ Summarization of the baseline algorithms. } }\label{tab:baseline_characteristic}
\vspace{-2mm}

  %\begin{tabular}{ c|c|c|c|c|c|c|c|c|c|c|r}%\label{tab:baseline_characteristic}
  \begin{tabular}{Sl|c|c|c|c|c|c|c|c|c|c|c}
    \toprule
    Characteristics&This work&FH&SH&KT&NNMF&MCA&LDA&LSA&PCA&$\chi^2$&MI\\
    \midrule
\pbox{5em}{Output\\ discrete\\ sketch}&\cmark&\cmark&\cmark&\cmark&\xmark&\xmark&\xmark&\xmark&\xmark&\cmark&\cmark\\ [0.5ex]
\hline
\pbox{5em}{Output\\ real-valued\\ sketch}&\xmark&\xmark&\xmark&\xmark&\cmark&\cmark&\cmark&\cmark&\cmark&\xmark&\xmark\\
\hline
\pbox{5em}{Approximating\\ distance\\ measure}&{Hamming}&\pbox{4em}{ Dot\\product}& {Cosine}& \texttt{NA} &\texttt{NA} &\texttt{NA} &\texttt{NA} & \texttt{NA}& \texttt{NA} &\texttt{NA} &\texttt{NA} \\
%&\texttt{distance}&\texttt{ product}& \texttt{Similarity}&  & & & & & & & \\
\hline
\pbox{5em}{Require \\labeled data}&\xmark&\xmark&\xmark&\xmark&\xmark&\xmark&\xmark&\xmark&\xmark&\cmark&\cmark\\
\hline
\pbox{5em}{Dependency\\ on the size\\ of sample \footnotemark} &\xmark&\xmark&\xmark&\xmark&\xmark &\cmark&\xmark&\cmark &\cmark&\xmark &\xmark\\
\hline 
\pbox{5em}{End tasks\\ comparison}&All&All&All&All& \pbox{5em}{Clustering,\\ Similarity Search,\\ Classification}
&\pbox{5em}{Clustering,\\ Similarity Search,\\ Classification}
&\pbox{5em}{Clustering,\\ Similarity Search,\\ Classification}
&\pbox{5em}{Clustering,\\ Similarity Search,\\ Classification}
&\pbox{5em}{Clustering,\\ Similarity Search,\\ Classification}
&Classification&Classification\\
\bottomrule
 \end{tabular}

\end{table*}

\footnotetext[9]{\footnotesize{The size of the maximum possible reduced dimension is the minimum of the number of data points and the dimension.}}

  \subsection{Reproducibility details for clustering task:}\label{appendix:clustering}. As our dataset is discrete and we measure the similarity between data points using Hamming distance, we use a discrete clustering algorithm -- $k$-mode~\cite{kmode} to compute the ground truth clustering results on the full-dimensional data. We use the following implementation for $k$-mode algorithm \footnote{\url{https://pypi.org/project/kmodes/}}. We then reduce the dimension of data using several baselines. Some of our baseline algorithms output discrete sketches, and the remaining output real-valued sketches. We, therefore, use different clustering algorithms, to measure the clustering quality on the respective sketches. We discuss it as follows: {Feature Hashing}~\cite{WeinbergerDLSA09}, {SimHash}\cite{simhash}, and {Kendall rank correlation coefficient}\cite{kendall1938measure} output integer/discrete  sketches.  Therefore we use the    $k$-mode algorithm on their sketches to evaluate the clustering results. Whereas, {Latent Semantic Analysis (LSA)}~\cite{LSI}, {Latent Dirichlet Allocation (LDA)}~\cite{LDA}, {Non-negative Matrix Factorization (NNMF)}~\cite{NNMF},  {Principal component analysis (PCA)}, and {Multiple Correspondence Analysis (MCA)}~\cite{MCA} output real-valued sketches. Therefore, we use the $k$-means algorithm on the low-dimensional datasets to evaluate the clustering results. We use implementation available in \texttt{sklearn} library for $k$-means\footnote{\url{https://scikit-learn.org/stable/modules/classes.html\#module-sklearn.cluster}}. For both $k$-mode and $k$-means algorithms, use the value of \texttt{random\_state = 42}. We then compare the quality of the clustering result \textit{via} \textit{purity index}. We define it as follows:
Let $m$ be the number of data points;  $\Omega=\{\omega_1, \omega_2,\ldots, \omega_k\}$ be the set of 
   clusters obtained on the original data; and $\mathcal{C}=\{c_1, c_2,\ldots, c_k\}$ be a set of 
   clusters obtained on reduced dimensional data. Then \textit{purity index} of clusters $\mathcal{C}$ is defined as
 
\[
   \textit{purity index}(\Omega, \mathcal{C})=\frac{1}{m}\sum_{i=1}^k \max_{1\leq j\leq k}|\omega_i \cap  c_j|.
  \]

\subsection{Reproducibility details for the classification task:} We use \texttt{logistic regression} classifier, and we use its implementation available in \texttt{sklearn} library \footnote{\url{https://scikit-learn.org/stable/modules/classes.html\#module-sklearn.linear_model}}. We use the value of \texttt{random\_state = 42} in the function for the classifier.
